# Supplementary material for: Large-Scale Meta-Learning with Continual Trajectory Shifting
Source: arXiv:2102.07215 source file (2022-02-16)
Supplement: Supplementary file 6 [file table2.tex]

\begin{table}[H]
\centering
\small
  \caption{\small\textbf{Test classification accuracies (\%)} when we let each target dataset contain only 1,000 images. We report the mean accuracies and the $95\%$ confidence intervals over 5 runs.}
  \vspace{0.05in}
  \resizebox{1.\linewidth}{!}{
 \begin{tabular}{c | c c c c c c c c c c}
 \hline
  ImageNet & \multicolumn{8}{c}{Target dataset} \\
pre-training & Dogs & Cars & Pets & Flowers & Food-101 & Aircraft & CUB & SUN397 & DTD \\
 \hline
 \hline
+ None
& 55.56\tiny$\pm$0.29 % dogs
& 23.15\tiny$\pm$0.27 % cars
& 83.48\tiny$\pm$0.15 % pets
& 87.01\tiny$\pm$0.38 % flowers
& 36.95\tiny$\pm$0.37 % food
& 33.43\tiny$\pm$0.29 % aircraft
& 34.32\tiny$\pm$0.46 % cub
& 29.62\tiny$\pm$0.24 % sun
& 59.39\tiny$\pm$0.53 % dtd
\\

+ MTL
& 55.00\tiny$\pm$0.28 % dogs
& \bf 23.82\tiny$\pm$0.19 % cars
& 83.29\tiny$\pm$0.25 % pets
& 87.04\tiny$\pm$0.34 % flowers
& 36.84\tiny$\pm$0.37 % food
& 34.02\tiny$\pm$0.55 % aircraft
& 34.19\tiny$\pm$0.88 % cub
& 29.30\tiny$\pm$0.28 % sun
& 58.86\tiny$\pm$0.49 % dtd
\\

+ Reptile
& 56.97\tiny$\pm$0.12 % dogs
& 22.49\tiny$\pm$0.40 % cars
& 84.25\tiny$\pm$0.22 % pets
& 87.22\tiny$\pm$0.31 % flowers
& 37.35\tiny$\pm$0.22 % food
& 33.81\tiny$\pm$0.35 % aircraft
& 35.44\tiny$\pm$0.48 % cub
& 29.37\tiny$\pm$0.29 % sun
& 58.98\tiny$\pm$0.59 % dtd
\\

\hline
\bf + Ours
& \bf 57.53\tiny$\pm$0.48 % dogs
& 23.80\tiny$\pm$0.40 % cars
& \bf 84.65\tiny$\pm$0.11 % pets
& \bf 87.54\tiny$\pm$0.21 % flowers
& \bf 37.84\tiny$\pm$0.20 % food
& \bf34.42\tiny$\pm$0.48 % aircraft
& \bf 36.40\tiny$\pm$0.20 % cub
& \bf 29.74\tiny$\pm$0.08 % sun
& \bf 59.53\tiny$\pm$0.25 % dtd

\\

\hline
\end{tabular}
}

  \label{tbl:imagenet}
  \vspace{-0.15in}
\end{table}
